# Supplementary material for: Quantizable Transformers: Removing Outliers by Helping Attention Heads Do Nothing
Source: arXiv:2306.12929 source file (2023-11-09)
Supplement: Supplementary file 1 [file E_code.tex]

\section{Code}
\label{app:code}

Idea: put a code snippet for implementation of our methods (to show how simple modifications are).
