# Supplementary material for: Quantizable Transformers: Removing Outliers by Helping Attention Heads Do Nothing
Source: arXiv:2306.12929 source file (2023-11-09)
Supplement: Supplementary file 2 [file _C_proofs.tex]

\section{Proofs}
\label{app:proofs}
% 

Proofs of statements regarding properties of the softmax mentioned in the Analysis section.
